# Supplementary material for: Scattering makes a difference in circular dichroic angle-resolved photoemission
Source: arXiv:2410.19652 source file (2024-10-25)
Supplement: Supplementary file 1 [file Boban_supplement.pdf]

# Supplementary Information

Honey Boban,[1,2] Mohammed Qahosh,[1] Xiao Hou,[1,2] Tomasz Sobol,[3] Edyta Beyer,[3] Magdalena Szczepanik,[3] Daniel Baranowski,[1] Simone Mearini,[1] Vitaliy Feyer,[1] Yuriy Mokrousov,[4,5] Keda Jin,[6,2,7] Tobias Wichmann,[6,2,8] Jose Martinez-Castro,[6] Markus Ternes,[6,7] F. Stefan Tautz,[6,8] Felix Lüpke,[6] Claus M. Schneider,[1,9,10] Jürgen Henk,[11] and Lukasz Plucinski[1,7,*]

[1] *Peter Grünberg Institut (PGI-6), Forschungszentrum Jülich GmbH, 52428 Jülich, Germany*
[2] *JARA-FIT (Fundamentals of Future Information Technology), Jülich-Aachen Research Alliance, Forschungszentrum Jülich and RWTH Aachen University, 52425 Jülich, Germany*
[3] *National Synchrotron Radiation Centre SOLARIS, Jagiellonian University, Kraków, Poland*
[4] *Peter Grünberg Institut (PGI-1), Forschungszentrum Jülich GmbH, 52428 Jülich, Germany*
[5] *Institute of Physics, Johannes Gutenberg University Mainz, 55099 Mainz, Germany*
[6] *Peter Grünberg Institut (PGI-3), Forschungszentrum Jülich GmbH, 52428 Jülich, Germany*
[7] *Institute for Experimental Physics II B, RWTH Aachen University, 52074 Aachen, Germany*
[8] *Institute for Experimental Physics IV A, RWTH Aachen University, 52074 Aachen, Germany*
[9] *Fakultät für Physik, Universität Duisburg-Essen, 47048 Duisburg, Germany*
[10] *Physics Department, University of California, Davis, CA 95616, USA*
[11] *Institut für Physik, Martin-Luther-Universität Halle-Wittenberg, 06099 Halle (Saale), Germany*
(Dated: October 25, 2024)

## SI. FINAL STATES IN ATOMIC PHOTOIONIZATION FROM $Y_1^0$ ORBITAL OF GRAPHENE, WITH AND WITHOUT MUTIPLE SCATTERING

Let us consider a spherically-symmetric potential. For such potential bound wave functions can be factorized into radial and angular parts, $\phi_{nlm} = R_{nl} \cdot Y_l^m$. Free (scattering) states can be written as a partial wave expansion, with a radial part not depending on quantum number $m$ (see e.g. [1]). Optical dipole matrix element only allows $l \pm 1$ transitions. Therefore, in cases where only $l+1$ channel exists, the photoionization final state from $\phi_{nlm}$ with $C_\pm$ light has an angular profile $Y_{l+1}^{m\pm1}$. For $Y_1^0$ orbital, with the light incident along the $z$-axis with $C_\pm$ the photonionization profiles are $Y_2^{\pm1}$. The angular dependence and phases of these profiles are shown in Fig. S1 (a)-(b). Both $Y_2^{-1}$ and $Y_2^1$ profiles, when squared, result in the same intensity profile shown in (c) as a map of the emission over the upper half space. This means that CDAD vanishes in this geometry.

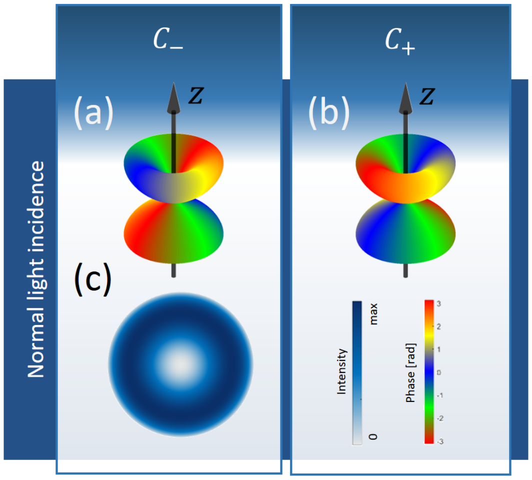


FIG. S1. Final states of the atomic photoionization from $Y_1^0$ orbital at normal light incidence, that is along the $z$-axis. (a) Final state with $C_-$ (LCP) excitation, which has a form of $Y_2^{-1}$. (b) Same by with $C_+$ (RCP). (c) Intensity profile related to both (a) and (b). Inset shows color scales.

* l.plucinski@fz-juelich.de

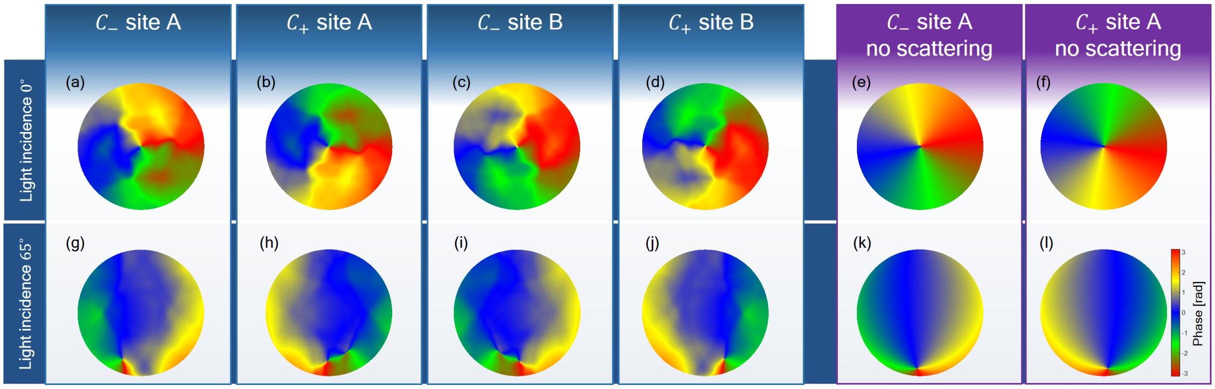


FIG. S2. (a)-(d) Complex phases of the final state wave functions related to main text Fig. 3 (a)-(d), $\theta_{h\nu} = 0°$. (e)-(f) Same as (a)-(b) but for final state without scattering, therefore identical to upper half space phases of $Y_2^{-1}$ and $Y_2^1$ complex spherical harmonics. (g)-(l) Same as (a)-(f) but for $\theta_{h\nu} = 65°$. Inset in (l) relates the color code to the complex phase, the color assignment is blue: 0, green: $-\pi/2$, yellow: $\pi/2$, and red: $\pm\pi$. All panels were calculated using the EDAC code [2] for $h\nu = 40$ eV, assuming $h\nu = E_{kin} + 6$ eV.

Fig. 3 (a)-(b) of main text shows intensities related to emissions from sites $A$ and $B$ of graphene and $\theta_{h\nu} = 0°$, with multiple scattering included. Figure S2 (a)-(d) shows related phases. Fig. S2 (e)-(f) shows phases without multiple-scattering, this is essentially a top view on profiles in Fig. S1 (a)-(b).

Figure S2 (g)-(j) shows the phases related to the intensities at $\theta_{h\nu} = 54.7°$ shown in Fig. 3 (g)-(j) of the main text. Figure S2 (k-l) shows related phases without multiple scattering.

One can see that scattering causes scrambling of the atomic-like phases of Fig.S2 (e)-(f) and (k)-(l). Since emissions from sites $A$ and $B$ are added coherently, these phases lead to interferences in matrix element calculations. Since, in particular at higher photon energies, band features are often confined to narrow angle ranges, this visualizes difficulties in recovering initial state OAM from CD-ARPES maps.

The independent atomic center approximation (IACA) takes into account atomic-like photoionization profiles, but not the effects of multiple scattering. It was first defined by Grobman [3] and later used by Schattke et al. [4], Moser [5], Day et al. [6] and others. These formulations considered either free states of the localized Coulomb photohole or the free-states of the muffin tin potential of the emitter atom. The real-space approach to angle-resolved photoemission is rooted in the work pioneering of Liebsch [7]. In the context of dispersive bands, augmenting IACA with multiple scattering has been introduced by Krüger et al. [8].

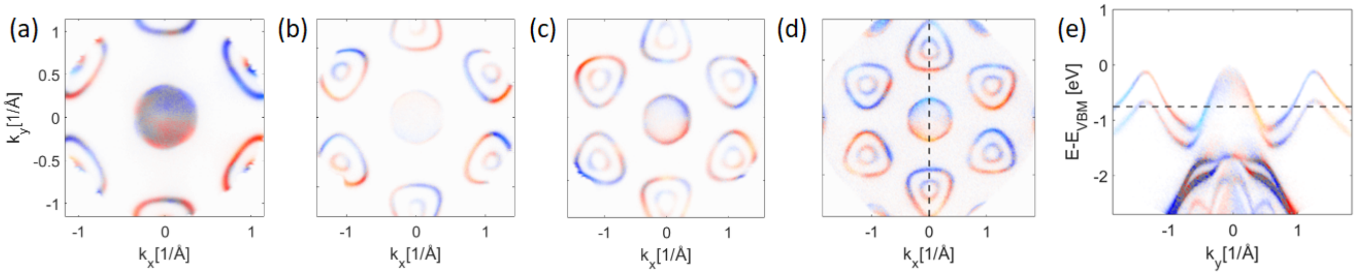


FIG. S3. Experimental CD-ARPES constant energy maps centered at normal emission from bulk $WSe_2$ at $h\nu$ = (a) 80 eV, (b) 120 eV, (c) 150 eV and (d) 200 eV. Spectra were taken on one of the terraces at $\theta_{h\nu} = 54.7°$. In all cases a full 3D set of data has been taken over $\approx 3$ eV binding energy range, as shown in (e). We use the valence band maximum at the $K/K'$ point $E_{VBM@K}$ as a reference, since bands at $K/K'$ are known to exhibit very small perpendicular dispersion and are well defined in our spectra. The shown cuts are at the kinetic energy $E_{VBM@K} - 0.725$ eV, as shown by the dashed line in (e). The same colormap as in Fig. 1 of the main text has been used.

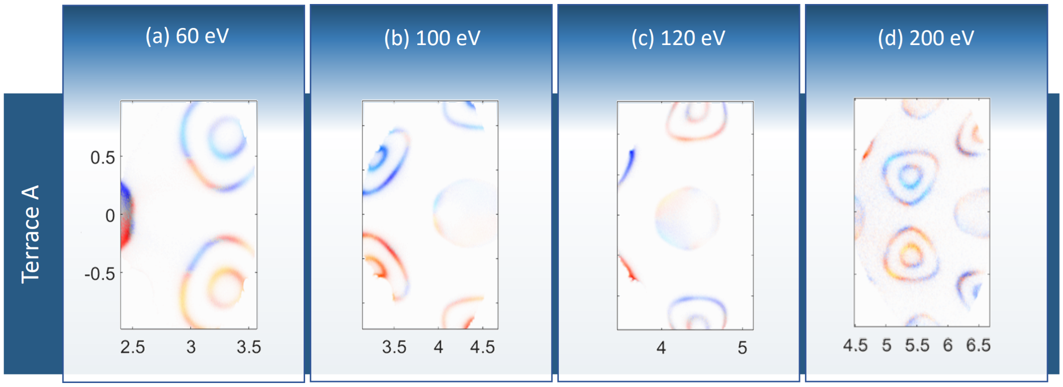


FIG. S4. Experimental normal incidence CD-ARPES spectra on bulk $WSe_2$ at $h\nu$ = (a) 60 eV, (b) 100 eV, (c) 120 eV and (d) 200 eV. The shown cuts are at the kinetic energy $E_{VBM@K} - 0.725$ eV. The same colormap as in Fig. 1 of the main text has been used.

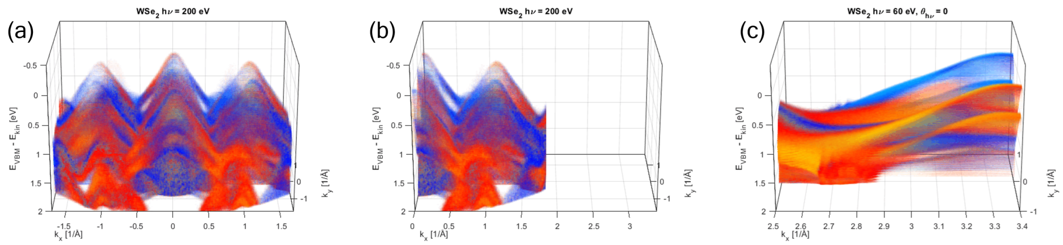


FIG. S5. 3D representation of selected $WSe_2$ CD-ARPES maps. In all cases the first frame of the animated GIF files (attached to the submission) is shown. (a) The 3D that has been used to produce Fig. 1 (g) of the main text and Fig. S3-(d)-(e). (b) Same as (a), but with smaller $k_x$ range to visualize the bands at $K/K'$. The 3D set that has been used to produce main text Fig. 6 (a)(f)(g) and Fig. S4 (a). The same colormap as in Fig. 1 of the main text has been used. Animated GIF file names are (a): WSe2_200eV_animated.gif, (b): WSe2_200eV_animated_cut_kx_0.gif, (c): WSe2_60eV_animated_normal_inc.gif.

## SII. ADDITIONAL $WSe_2$ CD-ARPES SPECTRA

Figures S3 and S4 show $WSe_2$ spectra taken at various photon energies. In practically all cases complex CD patterns are observed with CD sign changes within the $K/K'$ contours. Therefore, these patterns cannot be considered as a probe of initial state OAM of the W 5d orbitals at $K/K'$.

We have prepared animated GIF files visualizing our CD-ARPES data. First frames of the animations are shown in Fig. S5, see caption for details.

Figure S6 shows set of PED patterns from $Y_2^{\pm 2}$ orbitals of outermost W atom in $WSe_2$ at different photon energies. Maps calculated using EDAC [2] without (scattering order 0) and with (scattering order 30) multiple scattering

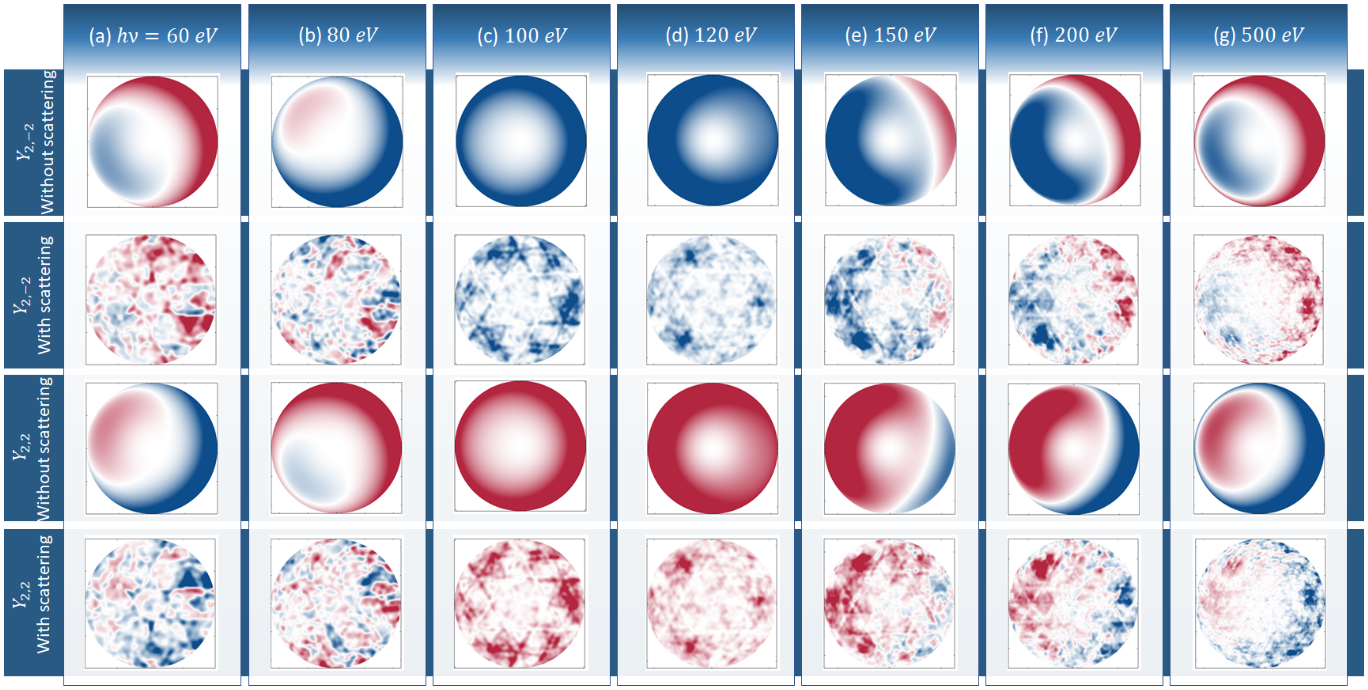


FIG. S6. Calculated circular dichroic patterns of $WSe_2$ using EDAC code for initial state taken as W $5d_{2,-2}$ (first and second rows) and W $5d_{2,2}$ (third and fourth rows), without multiple scattering (first and third rows) and with multiple scattering (second and fourth rows) at photon energies (a) 60 eV, (b) 80 eV, (c) 100 eV, (d) 120 eV, (e) 150 eV, (f) 200 eV and (g) 500 eV. We used spherical cluster with radius of $R_{max}$ = 15 Å, with 463 atoms spread through 3 layers of $WSe_2$, with IMFP of 5 Å, and with $\theta_{h\nu} = 54.7°$. Each pattern shows the full half space emission above the surface.

are shown, which enables to visually inspect the influence of multiple scattering. At $h\nu$ between 100 and 120 eV calculations predict no sign reversals of the CD over the the entire emission pattern. This would suggest that at these energies CD-ARPES experiment could be able to probe initial state OAM, and the sign of CD of the $K/K'$ contours should alternate between $K$ and $K'$ regions. This is not observed in experiment.

As shown in Figs. S7 and S8 the orbital characters near $K/K'$ points are mixed between W 5d and Se 4p (contributions from W 6$s$ and Se 4$s$ orbitals are small and can be neglected). This calculation has been performed using WIEN2k [9], an LAPW package that divides the space into atom-centered muffin tin potentials and regions in between. What is plotted in these figures is the charge contribution at each eigenvalue within the respective muffin-tin sphere that represents W and Se atoms. In WIEN2k calculation radiuses of these muffin tin spheres were 2.45 Bohr for W and 2.33 Bohr for Se. Approximately 0.73 of the W 5d electron and 0.59 of the Se 4p electron has been enclosed within their muffin tin spheres. At the same time, at $K/K'$ points the W 5d $Y_2^{\pm 2}$ contribution is 0.51 and 0.47 for the upper and lower spin-split band, while Se 4p $Y_1^{\pm 1}$ contribution is 0.06 and 0.07 respectively (these are values for bulk $WSe_2$ at $k_z = 0$, we also checked that values for $WSe_2$ monolayer are very similar). One can in principle correct these numbers by the above-mentioned occupancy within muffin tin spheres, which will increase the relative Se 4p contribution that can finally be estimated at 10-20% of that of W 5d $Y_2^{\pm 2}$. Furthermore, Se atoms contribute significantly more to the photoemission signal due to few Å inelastic mean free path (IMFP) at the considered energies. On top of that, one needs to consider orbital photoionization cross sections which we plotted in Fig. S9. One can see that at cross sections of W 5d and Se 4p meet at $E_{kin} \approx 130$, below that energy W 5d dominates and above Se 4p dominates.

Furthermore, also other layers of W and Se atoms will contribute a non-vanishing signal, and all these contributions should be coherently combined, although in practice the signal from the second layer W atoms might already be nearly vanishing.

Taking all this into account, we conclude that near $K/K'$ signal due to Se 4p $Y_1^{\pm 1}$ can be significant near $K/K'$, for $h\nu > 100$ eV, and perhaps even dominating for $h\nu$ between 150 and 300 eV. Nevertheless, for clarity, in the main text we only analyzed emission from W 5d $Y_2^{\pm 2}$ since it illustrates the key mechanisms governing the CD-ARPES process near the $K/K'$ points of $WSe_2$.

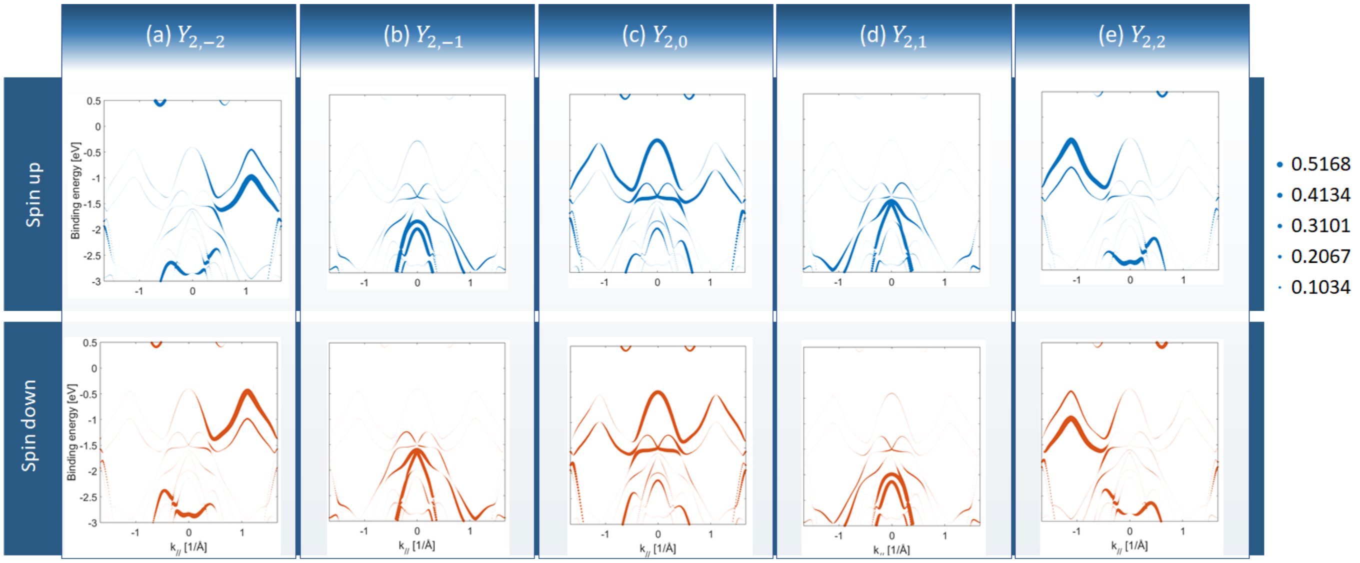


FIG. S7. $Y_{lm}$ decomposition of the W $d$ orbitals of $WSe_2$ along $M-K-\Gamma-K'-M$ direction. The spin up and spin down bands are shown in the top and bottom panels respectively. Calculation performed using WIEN2k [9].

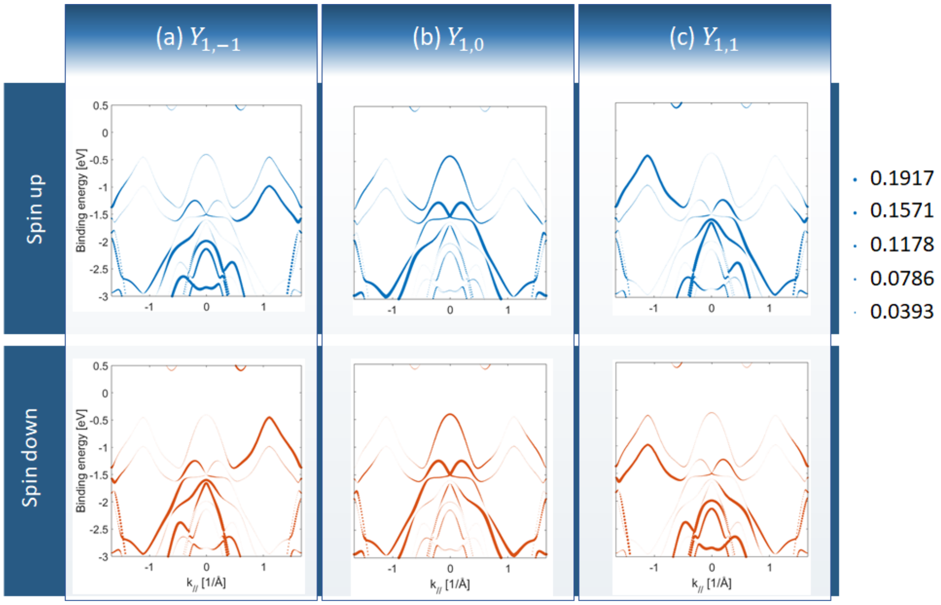


FIG. S8. $Y_{lm}$ decomposition of the Se $p$ orbitals of $WSe_2$ along $M-K-\Gamma-K'-M$ direction. The spin up and spin down bands are shown in the top and bottom panels respectively. Calculation performed using WIEN2k [9].

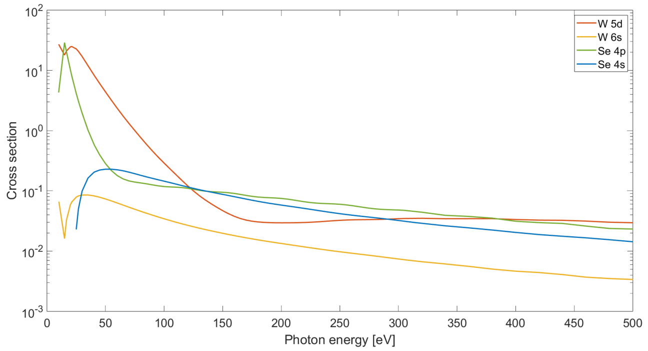


FIG. S9. Photoionization cross section of W 5$d$, W 6$s$, Se 4$p$ and Se 4$s$

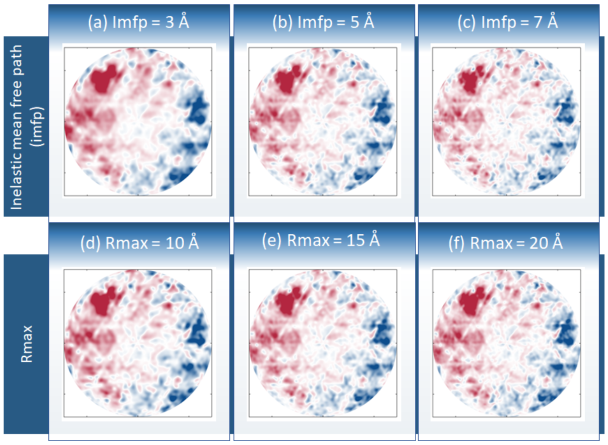


FIG. S10. Calculated circular dichroic patterns of $WSe_2$ using EDAC code for initial state taken as W $5d_{2,2}$ with inelastic mean free path (IMFP) (a) 3 Å, (b) 5 Åand (c) 7 Å, with scattering order = 30 and $R_{max}$ = 15. Similar calculations with IMFP = 5 Å, scattering order = 30 and $R_{max}$ = (d) 10 Å, (e) 15 Åand (f) 20 Å.

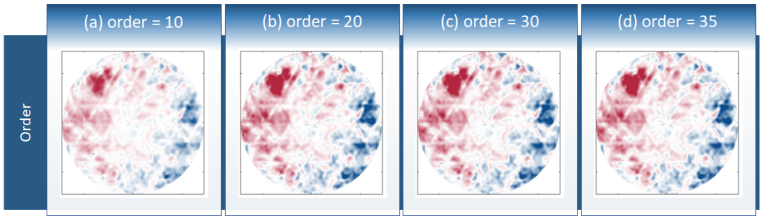


FIG. S11. Calculated circular dichroic patterns of $WSe_2$ using EDAC code for initial state taken as W $5d_{2,2}$ with inelastic mean free path (IMFP) = 5 Å, $R_{max}$ = 15 and scattering order = (a) 10, (b) 20, (c) 30 and (d) 35.

## SIII. TECHNICAL DETAILS ON EDAC CALCULATIONS

Our PED calculations were performed using the EDAC code which is described in Ref. [2]. All presented calculations were made using the *recursion* method. Figures S10 and S11 show W 5d $Y_2^2$ PED CD patterns calculated with EDAC at different settings. Figure S10 demonstrates that CD patterns exhibit no significant changes when the IMFP is varied between 3 and 7 Å, and that at IMFP of 5 Å the radius of the cluster of $R_{max}$ = 15 Å is sufficient. Figure S11 shows that convergence in the calculations is reached at the scattering order 20.

Similar tests were performed for graphene with the same conclusions.

All maps were calculated in 1° step in both polar and azimuthal angles. For $WSe_2$ a single PED map at $R_{max}$ = 15 Å and scattering order 30 takes a few minutes to calculate on a modern desktop PC running Linux.

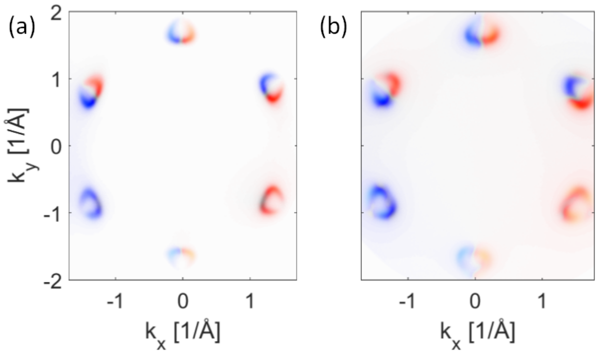


FIG. S12. Experimental CD-ARPES spectra on (a) hBN/graphene and (b) graphite at $h\nu = 40$ eV. The constant energy cut is at $E_B = 1.25$ eV.

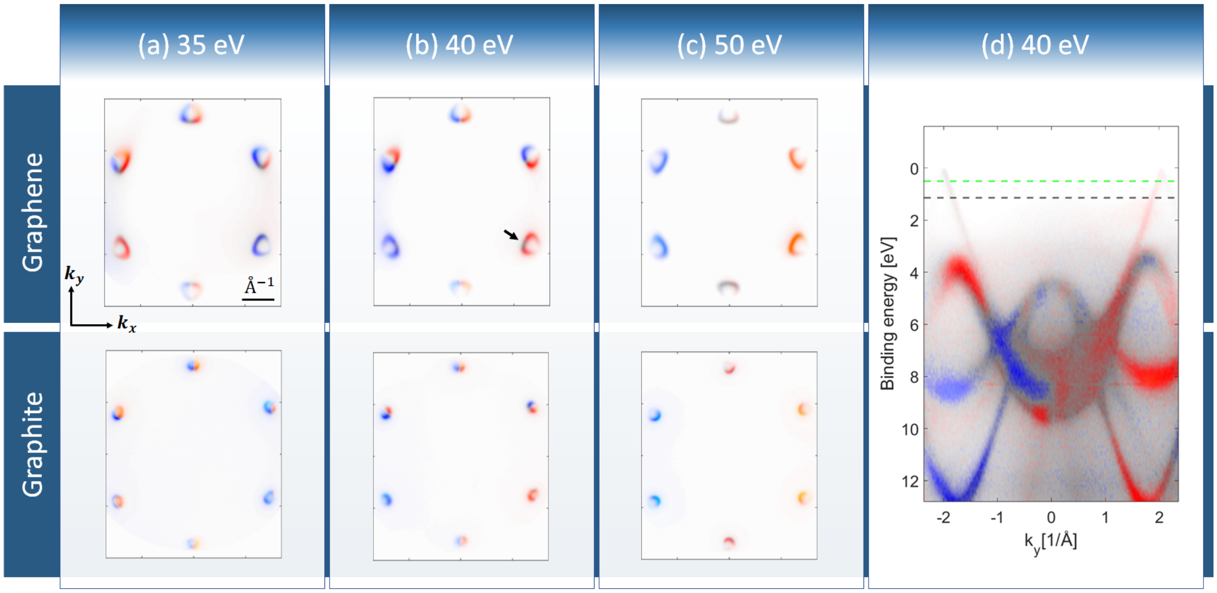


FIG. S13. Experimental CD-ARPES spectra from graphene (top panel) and graphite (bottom panel) at $h\nu =$ (a) 35 eV, (b) 40 eV and (c) 50 eV. (d) shows the $E_B$ vs $k_y$ CD map of graphene/hBN at $h\nu = 40$ eV. The maps (a)-(c) show constant energy cuts at $E_B = 1.25$ eV (black line in (d)) for graphene and $E_B = 0.5$ eV (green line in (d), shown for orientation) for graphite. Black arrow in (b) indicates a region where small deviation from the perfect $\mathcal{M}_x$ mirror symmetry occurs, this is likely due to the effect of the hBN substrate.

## SIV. COMPARISON OF CD-ARPES FROM GRAPHENE AND GRAPHITE

Figures S12 and S13 compare CD-ARPES maps from graphene/hBN and graphite. The maps are quantitatively similar, therefore the behavior of CD-ARPES pattern is a robust property of graphene and is not related to the hBN substrate.

A detailed inspection reveals that spectra from graphite do not fully obey the $\mathcal{M}_x$ mirror plane. The reason is that $\mathcal{M}_x$ is a mirror plane of graphene but not of graphite. Graphene (space group $P\bar{6}m2$ No. 187) has 6 vertical mirror planes while graphite (space group $P6_3mc$, No. 186) has 3 vertical mirror planes.

Furthermore, the $\mathcal{M}_x$ mirror plane is not expected to hold perfectly also in our graphene data due to the scattering from the hBN substrate. A small region where such asymmetry is likely present is indicated by the black arrow in Fig. S13 (b). As shown in Fig. S14, the we estimate the twist angle between graphene and hBN to be around 20°, which a generic value. In case of graphite no substrate is present, therefore quantitative agreement between graphite and graphene CD-ARPES maps demonstrates that the overall character of our CD-ARPES maps does not depend on the hBN substrate. Most important, energy-dependent CD sign inversions of different Dirac contours are the same for graphene and graphite.

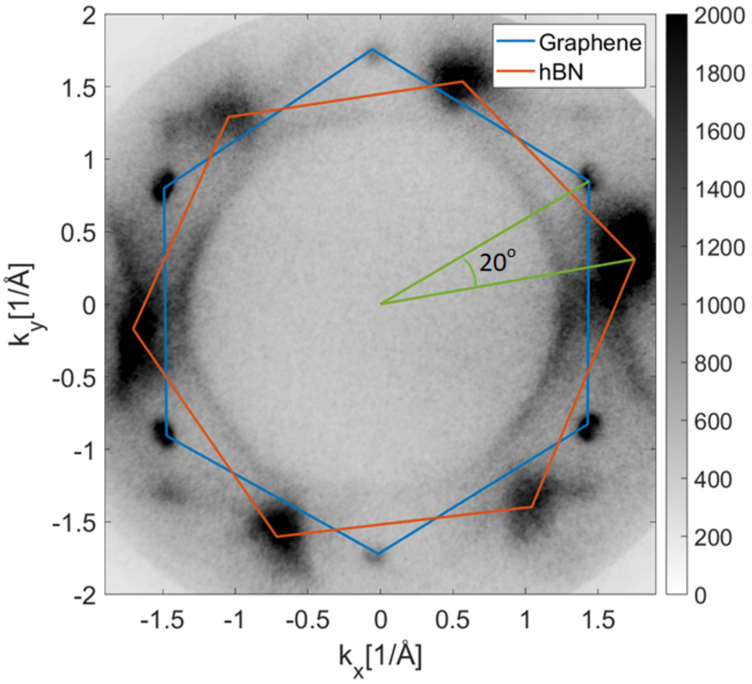


FIG. S14. Two superimposed constant energy cuts on hBN/graphene showing the Dirac cones of graphene at $E_B = 0.4$ eV and valence band maximum of hBN at $E_B$ =3.3.eV.

## SV. GRAPHENE MICROFLAKE

Figure S15 shows an optical micrograph of the graphene flake used for the measurements. The flakes were prepared using mechanical exfoliation technique and were assembled into a heterostructure using dry transfer technique with PDMS/PC stamps. The sample was then washed in chloroform to remove the PC film. 2 nm Au coated $SiO_2$, with 1 nm Ti used as a sticking layer between Au and $SiO_2$, was used as the final substrate. Before the ARPES measurements the microstructure was annealed at 300°C for 1 hour in ultra high vacuum to remove the water and hydrocarbons from the sample surface.

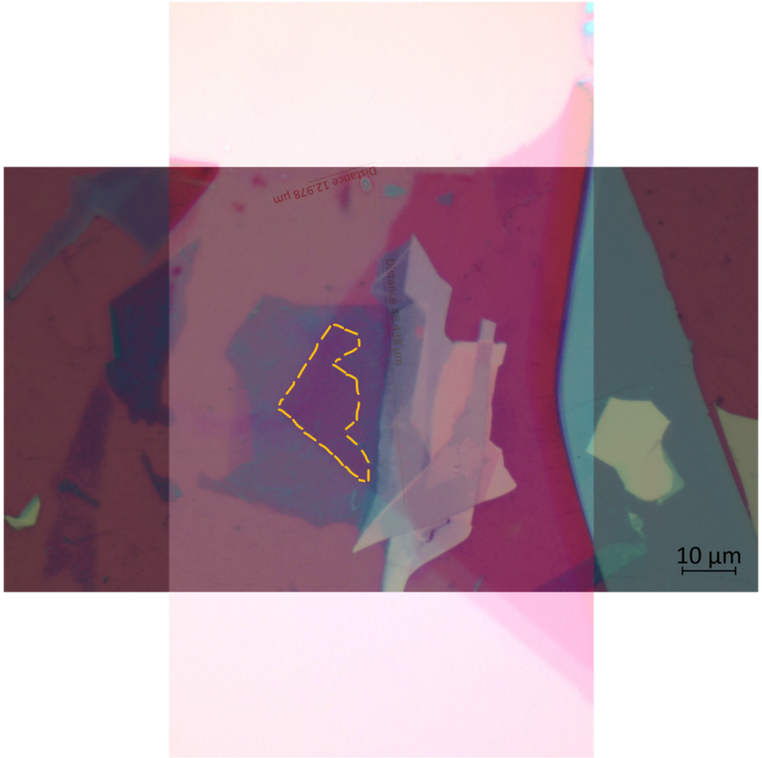


FIG. S15. Optical image of hBN/graphene flake used for the measurements in S12 (a). The monolayer graphene region is indicated in yellow dotted lines.

## SVI. RELATIONSHIP BETWEEN CD-ARPES AND XMCD

X-ray magnetic circular dichroism (XMCD) and CD-ARPES may be seen as similar techniques in a sense that in both cases circular light is used for excitation and emitted electrons are being measured. However, there also exist fundamental differences between the two techniques.

In CD-ARPES measured electrons have energies of $h\nu - E_B$ and their angular distribution is measured, with the final state being a scattering state (free state) of the electron outside the solid, the time-reversed LEED (TR-LEED) state. Relevant features in CD-ARPES are related to elastic electrons that did not lose energy between exciation and detection.

In XMCD the total electron yield, which contains primarily low energy electrons, is measured. Measurement is made at the absorption threshold of a core level and emitted electrons are primarily due to Auger cascades that subsequently exhibit inelastic scattering. In this scenario, the final state in the optical matrix element is assumed as a bound state within the solid, that can be approximated by a linear combination of atomic orbitals, which allows to avoid peculiarities of the TR-LEED state.

In XMCD all the information regarding the angular dependence in the interband optical transition is assumed to be lost, and one can consider measuring an angle-integrated average of initial excitation signal. This initial angle-dependent signal can be potentially similar to the one shown in Fig. 5 (f) of the main text, because it will involve transition between initial and final orbitals characterized by their respective $Y_l^m$.

Spin-orbit coupling (SOC) splits $l > 0$ core levels into doublets. The orbital weights within each feature of the doublet can be obtained by diagonalizing the $H_{SOC} = \mathbf{L} \otimes \mathbf{S}$ Hamiltonian, where $\otimes$ is a Kronecker product. For example $p$ orbitals split into $p_{3/2}$ and $p_{1/2}$, and each of these components is made from a linear combination of $Y_1^{-1}$, $Y_1^0$ and $Y_1^1$ spin-up and spin-down components. This gives 6 components in total, as we will show in the following.

Explicitly

$$\mathbf{S} = (\sigma_x, \sigma_y, \sigma_z) = \left( \begin{bmatrix} 0 & 1 \\ 1 & 0 \end{bmatrix}, \begin{bmatrix} 0 & i \\ -i & 0 \end{bmatrix}, \begin{bmatrix} 1 & 0 \\ 0 & 1 \end{bmatrix} \right) \tag{1}$$

is a vector of Pauli matrices, and for $l = 1$

$$\mathbf{L} = (L_x, L_y, L_z) = \left( \frac{1}{\sqrt{2}} \begin{bmatrix} 0 & 1 & 0 \\ 1 & 0 & 1 \\ 0 & 1 & 0 \end{bmatrix}, \frac{1}{\sqrt{2}} \begin{bmatrix} 0 & -i & 0 \\ i & 0 & -i \\ 0 & i & 0 \end{bmatrix}, \begin{bmatrix} 1 & 0 & 0 \\ 0 & 0 & 0 \\ 0 & 0 & -1 \end{bmatrix} \right) \tag{2}$$

is a vector of angular momentum matrices written in the basis of complex spherical harmonics, here in the order $Y_1^1$, $Y_1^0$, $Y_1^{-1}$. Then the Hamiltonian takes the form

$$H_{SOC} = \alpha \cdot \begin{pmatrix} Y_{1\uparrow}^1 & Y_{1\downarrow}^1 & Y_{1\uparrow}^0 & Y_{1\downarrow}^0 & Y_{1\uparrow}^{-1} & Y_{1\downarrow}^{-1} \\ \hline 1 & 0 & 0 & 0 & 0 & 0 \\ 0 & -1 & \sqrt{2} & 0 & 0 & 0 \\ 0 & \sqrt{2} & 0 & 0 & 0 & 0 \\ 0 & 0 & 0 & 0 & \sqrt{2} & 0 \\ 0 & 0 & 0 & \sqrt{2} & -1 & 0 \\ 0 & 0 & 0 & 0 & 0 & 1 \end{pmatrix} \tag{3}$$

where we also indicated the basis orbitals.

Diagonalization of this Hamiltonian leads to eigenvalues and wave functions listed in Fig. S16, and results in the $p_{1/2}$ $p_{3/2}$ doublet. One can check that the coefficients of the wave functions are the Clebsch-Gordan coefficients for $j_1 = 1$, $j_2 = 1/2$. The two wave functions $\psi_{1,2}$ represent the $p_{1/2}$ state, while the four $\psi_{3,4,5,6}$ represent the $p_{3/2}$ state.

Within the matrix element $\langle \psi_f | \mathbf{A} \cdot \mathbf{p} | \psi_i \rangle$ the magnetic sensitivity of XMCD is primarily achieved through considering transition between different orbital contributions of each of the doublet components and the spin-polarized final state at the Fermi level. In the simplified model, only $l + 1$ transition is considered, therefore the radial matrix element is the same for all transitions between participating orbitals and becomes a global proportionality constant, while angular matrix elements have analytical formulas [10].

A typical XMCD scenario is the transition between $2p$ and $3d$ levels of transition metals, where indeed near the Fermi level the weight of $3d$ levels is larger than the weight of $4s$ levels. If we consider CD-ARPES experiment from

| | $\psi_1$ | $\psi_2$ | $\psi_3$ | $\psi_4$ | $\psi_5$ | $\psi_6$ |
|---|---|---|---|---|---|---|
| Energy | -1 | -1 | 0.5 | 0.5 | 0.5 | 0.5 |
| $Y_{1\uparrow}^{1}$ | 0 | 0 | 0 | 0 | 0 | 1 |
| $Y_{1\uparrow}^{0}$ | $1/\sqrt{3}$ | 0 | 0 | 0 | $\sqrt{2/3}$ | 0 |
| $Y_{1\uparrow}^{-1}$ | 0 | $-\sqrt{2/3}$ | 0 | $1/\sqrt{3}$ | 0 | 0 |
| $Y_{1\downarrow}^{1}$ | $-\sqrt{2/3}$ | 0 | 0 | 0 | $1/\sqrt{3}$ | 0 |
| $Y_{1\downarrow}^{0}$ | 0 | $1/\sqrt{3}$ | 0 | $\sqrt{2/3}$ | 0 | 0 |
| $Y_{1\downarrow}^{-1}$ | 0 | 0 | 1 | 0 | 0 | 0 |

FIG. S16. Wave functions and eigenvalues of the $H_{SOC} = \mathbf{L} \otimes \mathbf{S}$ Hamiltonian for $l = 1$, Eq. 3, with $\alpha = 1$.

a SOC-split $2p$ level, then the final state is not anymore a well defined bound $3d$ orbital near the Fermi level, but a TR-LEED state, that in far field becomes a free-electron state.

One can also add exchange interaction $H_{ex} = 0.5 \cdot \Delta_{ex} \cdot I_3 \otimes \sigma_z$, and consider the total Hamiltonian $H_{SOC} + H_{ex}$ which will lead to further splittings within the initial state $\psi_{1/2}$ $\psi_{3/2}$ manifold (here $I_3$ is a $3 \times 3$ identity matrix), now with 6 different eigenvalues. With such exchange splitting, functions $\psi_3$ and $\psi_6$ are easiest to analyze since they remain purely $Y_{1\uparrow}^{1}$ and $Y_{1\downarrow}^{-1}$ while now being split in energy by $\Delta_{ex}$, which demonstrates a potential mechanism of magnetic sensitivity through CD-ARPES measurement. In a real material valence bands disperse (through an additional hopping term in the Hamiltonian) and band characters often significantly mix, therefore identification of magnetic signatures might require careful data analysis, in particular taking into account effects due to elastic scattering.

With all this taken into account, valence bands are often spin-orbit split and spin-polarized, such as at $K/K'$-points of $WSe_2$. In such situation one may consider a single well-defined $k$-dependent initial state orbital, which in case of $WSe_2$ is primarily $Y_2^{\pm 2}$ near $K/K'$. Even under IACA, in CD-ARPES this requires consideration of both $l \pm 1$ channels, where radial matrix elements need to be computed numerically and TR-LEED state is in effect, which leads to CD photoelectron diffraction patterns of Fig. 5 (g)-(h) of the main text. If a fully angle-integrated experiment would be possible, a net CD from $Y_2^2$ would be obtained (and similarly from $Y_2^{-2}$), which refers to the situation near $K$ ($K'$). In this paper we demonstrate that this picture is obscured by multiple scattering and by orbital character mixing at $K/K'$,


[1] S. Goldberg, C. Fadley, and S. Kono, Journal of Electron Spectroscopy and Related Phenomena **21**, 285 (1981).
[2] F. J. García de Abajo, M. A. Van Hove, and C. S. Fadley, Phys. Rev. B **63**, 075404 (2001).
[3] W. D. Grobman, Phys. Rev. B **17**, 4573 (1978).
[4] Section 2.7 in W. Schattke and M. A. Van Hove, eds., *Solid-state photoemission and related methods* (Wiley-VCH Verlag, Weinheim, Germany, 2003).
[5] S. Moser, Journal of Electron Spectroscopy and Related Phenomena **262**, 147278 (2023).
[6] R. P. Day, B. Zwartsenberg, I. S. Elfimov, and A. Damascelli, npj Quantum Materials **4**, 10.1038/s41535-019-0194-8 (2019).
[7] A. Liebsch, Phys. Rev. Lett. **32**, 1203 (1974).
[8] P. Krüger, F. Da Pieve, and J. Osterwalder, Phys. Rev. B **83**, 115437 (2011).
[9] P. Blaha, K. Schwarz, F. Tran, R. Laskowski, G. K. H. Madsen, and L. D. Marks, The Journal of Chemical Physics **152**, 074101 (2020), https://pubs.aip.org/aip/jcp/article-pdf/doi/10.1063/1.5143061/16727313/074101_1_online.pdf.
[10] J. Stohr and H. C. Siegmann, *Magnetism*, 2006th ed., Springer Series in Solid-State Sciences (Springer, Berlin, Germany, 2006).
